# Supplementary material for: When Blood Parts Ways: Phase Separation in Microstructured Environments
Source: arXiv:2509.01408 source file (2025-09-01)
Supplement: Supplementary file 1 [file supplementary_materials.pdf]

## Supplementary Information

### When Blood Parts Ways: Phase Separation in Microstructured Environments

Sampad Laha<sup>1,2</sup>, Ananta Kumar Nayak<sup>2</sup>, Alexander Farutin<sup>2</sup>, Suman Chakraborty<sup>1</sup>, Chaouqi Misbah<sup>2</sup>

<sup>1</sup> Department of Mechanical Engineering, Indian Institute of Technology, Kharagpur, India

<sup>2</sup> University of Grenoble Alpes, CNRS, LIPHY, F-38000, Grenoble, France.

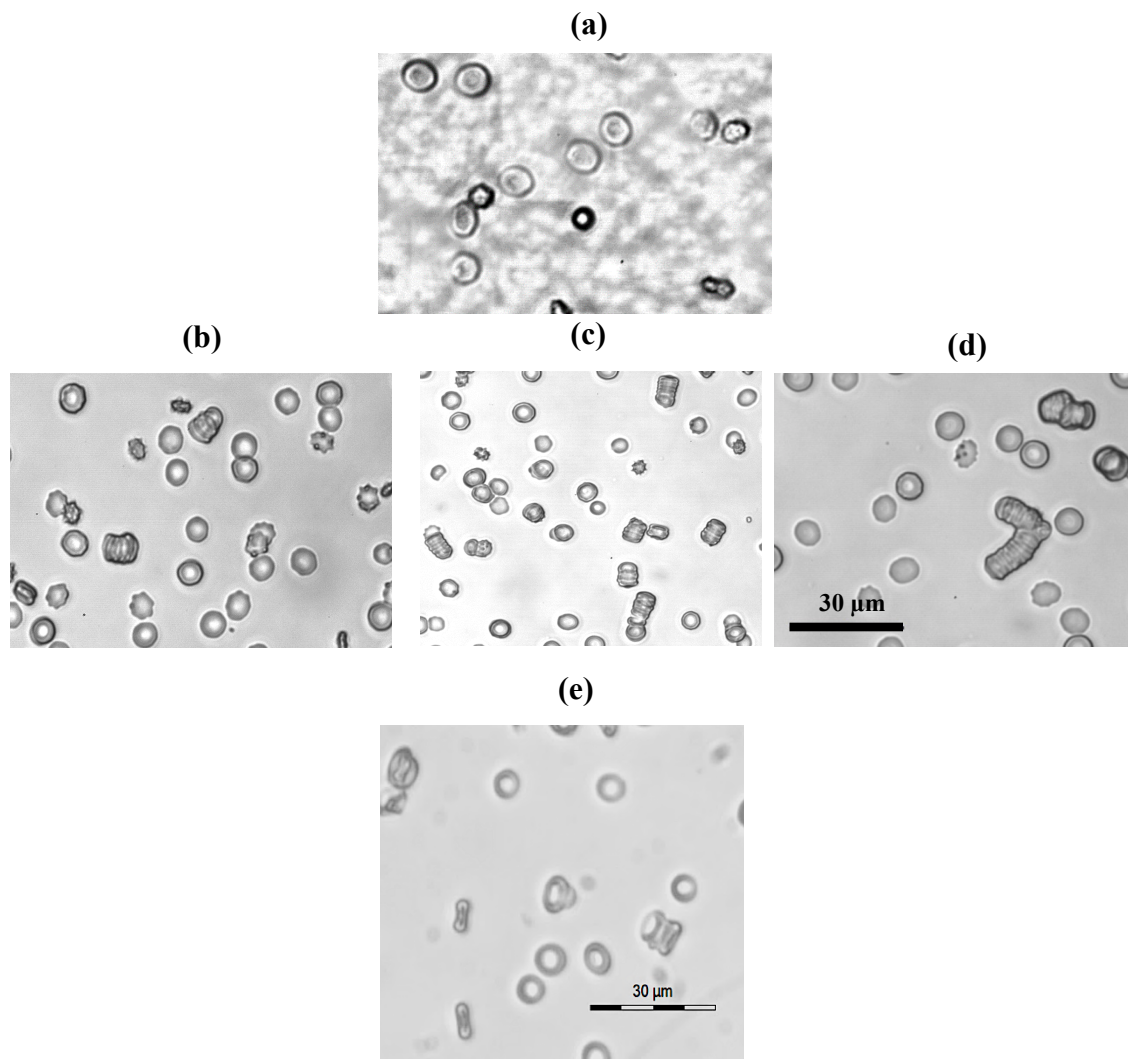

**Fig. S1:** Effect of dextran concentration on the structure of RBC aggregates as observed under brightfield mode in an inverted optical microscope (a) control case without dextran (b) dextran conc. 15 mg/ml (c) dextran conc. 30 mg/ml (d) dextran conc. 50 mg/ml. (e) shows smaller aggregates formed with rigid RBCs for dextran concentration 50 mg/ml, compared to larger complex aggregates in case of healthy RBCs for the same dextran concentration. All images captured for samples with HCT 2% over BSA-covered glass slides.

## Image processing for determination of phase separation area

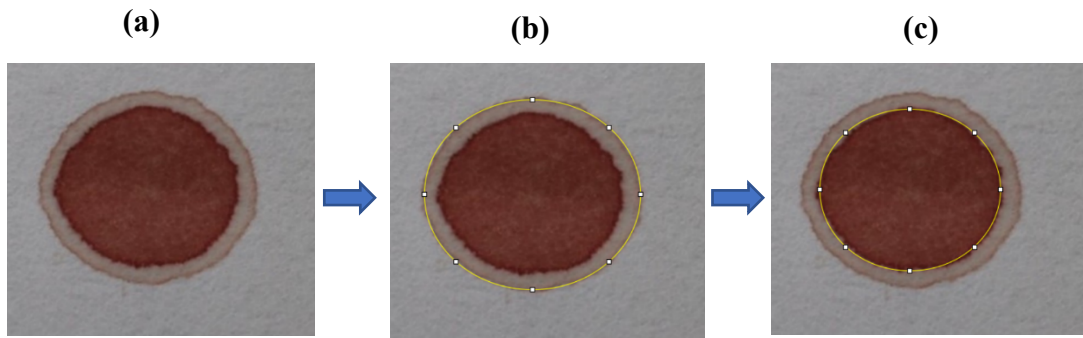

**Fig. S2:** *Image processing steps followed in ImageJ during determination of phases separation area of the blood patterns*

Image processing has been carried out using ImageJ software. At first, the blood pattern image is uploaded in the software (FigS2(a)). Thereafter, the average outer periphery of the phase separated region is fitted with a bounding shape using the ‘oval’ selection tool (FigS2(b)). The area of the selected region gives the total area of the blood pattern (including both RBC core region and phase separated region). Next, the area of the red core region is determined in a similar process (FigS2(c)). The difference between the above two values of the area gives the area of the phase separated region for each pattern. This area (in square pixels) is finally adjusted with appropriate calibration factors to deduce the area value in terms of standard units such as  $\text{mm}^2$ .
